# Supplementary material for: Ghost Echoes: Semantic Erasure Failure in Retrieval-Backed Applications
Source: arXiv:2608.20352 source file (2026-06-16)
Supplement: Supplementary file 1 [file 12_appendix.tex]

\section{Appendix}
\label{sec:appendix}

\subsection{Supporting Induction Evidence}
\label{app:induction}
Table~\ref{tab:legacy-ranks} reports the underlying median ranks achieved by our black-box induction mechanisms across backends. These ranks represent the semantic placement of the induction query within the corpus, supporting cross-backend induction viability.

\begin{table}[h]
\centering
\caption{Supporting cross-backend induction ranks (Medians over 18 targets).}
\label{tab:legacy-ranks}
\begin{tabular}{lccc}
\toprule
\textbf{Backend} & \textbf{Warm-Start Rank} & \textbf{NES Rank} & \textbf{Improvement} \\
\midrule
ChromaDB & 187 & 29 & 6.4$\times$ \\
FAISS & 1 & 1 & --- \\
Weaviate & 186 & 117 & 1.6$\times$ \\
Pinecone & 70 & 60 & 1.2$\times$ \\
\bottomrule
\end{tabular}
\end{table}

\subsection{Phantom Neighborhood: Passive Signal Boundary}
\label{app:phantom}
Our characterization of purely passive rank-drift (Phantom Neighborhood) is a boundary result showing scale-dependency. At $N=5,000$, we measure a mean Top-40 Jaccard drift of 0.18 [0.14, 0.22] following target deletion (Figure~\ref{fig:phantom-scale}). This establishes the boundary where passive signals emerge.

\begin{figure}[h]
\centering
\includegraphics[width=0.8\linewidth]{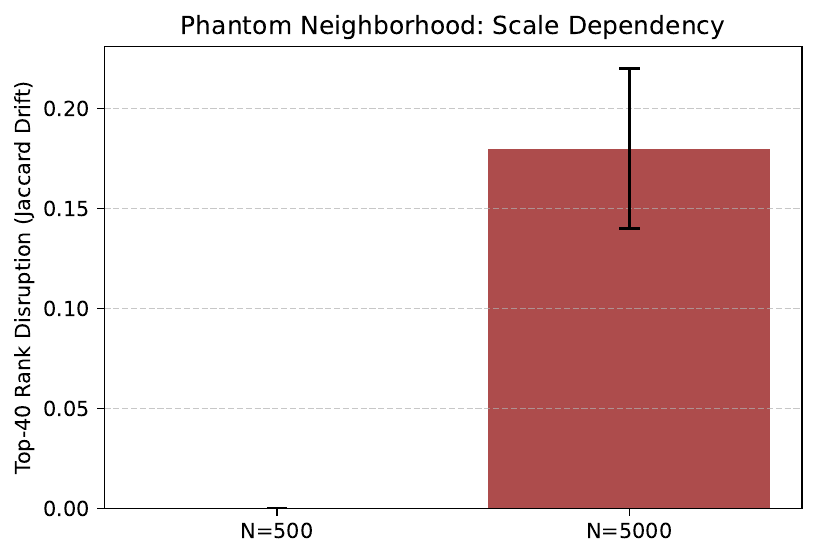}
\caption{Scale dependency of passive rank-only characterization. Rank disruption emerges at larger scales.}
\label{fig:phantom-scale}
\end{figure}
